# Supplementary material for: Dielectronic recombination studies on Fe$^{2+}$
Source: arXiv:2501.16987 source file (2025-03-25)
Supplement: Supplementary file 1 [file Supplementary-Data.pdf]

# Supplementary Data for Resonance Strength

| Energy (eV) | Width (eV) | Resonance Strength (barn*eV) | Energy (eV) | Width (eV) | Resonance Strength (barn*eV) | Energy (eV) | Width (eV) | Resonance Strength (barn*eV) |
|---|---|---|---|---|---|---|---|---|
| 0.022 | 1.379E-02 | 3.123E+04 | 0.514 | 1.814E-02 | 1.899E+02 | 1.070 | 1.326E-02 | 3.098E+02 |
| 0.037 | 8.267E-04 | 2.451E+04 | 0.517 | 7.433E-03 | 3.160E+01 | 1.071 | 1.318E-02 | 9.650E+01 |
| 0.043 | 3.544E-04 | 5.189E+04 | 0.518 | 3.615E-03 | 2.810E+01 | 1.074 | 2.689E-02 | 1.005E+03 |
| 0.044 | 2.988E-04 | 2.739E+04 | 0.534 | 4.460E-01 | 1.640E+03 | 1.075 | 4.792E-02 | 1.667E+03 |
| 0.045 | 9.878E-04 | 6.187E+04 | 0.547 | 3.054E-01 | 5.733E+02 | 1.075 | 9.045E-03 | 1.824E+03 |
| 0.046 | 3.428E-03 | 9.630E+04 | 0.559 | 9.786E-03 | 2.397E+01 | 1.083 | 1.014E-02 | 8.724E+02 |
| 0.048 | 1.510E-03 | 6.987E+04 | 0.569 | 2.752E-01 | 8.643E+01 | 1.088 | 3.777E-02 | 1.460E+03 |
| 0.050 | 2.626E-03 | 7.805E+04 | 0.587 | 2.582E-01 | 4.190E+00 | 1.105 | 2.697E-05 | 2.067E+02 |
| 0.050 | 3.979E-04 | 4.260E+03 | 0.594 | 2.240E-02 | 1.533E+03 | 1.120 | 9.090E-04 | 1.804E+02 |
| 0.071 | 4.061E-02 | 4.294E+03 | 0.605 | 8.578E-03 | 1.689E+01 | 1.121 | 2.323E-04 | 5.326E+02 |
| 0.097 | 2.968E-02 | 3.078E+03 | 0.623 | 1.020E-02 | 1.316E+02 | 1.127 | 2.627E-04 | 1.299E+02 |
| 0.105 | 2.000E-02 | 9.153E+02 | 0.639 | 9.109E-03 | 6.478E+01 | 1.129 | 8.559E-04 | 2.778E+01 |
| 0.116 | 8.368E-03 | 9.204E+02 | 0.645 | 8.111E-03 | 2.104E+03 | 1.138 | 1.345E-04 | 2.962E+01 |
| 0.118 | 1.348E-03 | 1.689E+04 | 0.646 | 2.055E-02 | 6.016E+01 | 1.142 | 7.017E-03 | 1.793E+02 |
| 0.118 | 2.839E-03 | 5.471E+02 | 0.646 | 1.258E-02 | 1.456E+03 | 1.142 | 6.962E-03 | 2.218E+01 |
| 0.121 | 4.513E-03 | 1.134E+04 | 0.651 | 1.499E-02 | 2.091E+02 | 1.144 | 6.790E-03 | 3.017E+03 |
| 0.122 | 3.203E-03 | 3.328E+03 | 0.654 | 1.163E-02 | 2.865E+03 | 1.146 | 7.054E-03 | 7.092E+02 |
| 0.123 | 4.508E-03 | 2.960E+02 | 0.659 | 9.993E-03 | 2.170E+03 | 1.169 | 3.490E-03 | 1.433E+03 |
| 0.125 | 1.273E-02 | 3.898E+04 | 0.661 | 9.190E-03 | 1.099E+03 | 1.182 | 2.899E-03 | 6.674E+02 |
| 0.128 | 1.292E-02 | 4.886E+01 | 0.664 | 6.940E-03 | 3.973E+02 | 1.203 | 1.815E-04 | 5.028E+02 |
| 0.129 | 1.327E-02 | 7.250E+02 | 0.670 | 1.536E-02 | 3.505E+03 | 1.212 | 3.978E-03 | 6.148E+02 |
| 0.130 | 1.338E-02 | 2.513E+02 | 0.674 | 9.551E-03 | 3.886E+01 | 1.220 | 2.388E-03 | 8.005E+01 |
| 0.130 | 1.284E-02 | 1.387E+03 | 0.677 | 2.099E-02 | 3.816E+03 | 1.221 | 3.537E-03 | 2.589E+02 |
| 0.132 | 1.268E-02 | 1.340E+04 | 0.679 | 1.463E-02 | 1.807E+01 | 1.226 | 2.987E-02 | 5.783E+02 |
| 0.132 | 1.277E-02 | 4.509E+03 | 0.692 | 1.613E-02 | 4.201E+01 | 1.237 | 2.797E-02 | 6.666E+02 |
| 0.147 | 1.760E-02 | 1.037E+02 | 0.714 | 1.785E-02 | 4.402E+01 | 1.302 | 1.983E-01 | 1.161E+03 |
| 0.162 | 8.863E-04 | 1.814E+04 | 0.781 | 2.460E-02 | 1.492E+00 | 1.320 | 8.606E-03 | 4.422E+01 |
| 0.163 | 2.009E-03 | 1.913E+02 | 0.806 | 2.201E-02 | 2.902E+02 | 1.323 | 5.989E-03 | 1.951E+03 |
| 0.164 | 2.580E-03 | 8.924E+02 | 0.822 | 2.002E-02 | 3.869E+02 | 1.324 | 9.576E-03 | 1.598E+03 |
| 0.165 | 7.257E-03 | 4.607E+03 | 0.947 | 1.023E-02 | 5.655E+02 | 1.325 | 1.041E-02 | 4.022E+02 |
| 0.165 | 1.787E-02 | 1.288E+04 | 0.952 | 1.118E-02 | 5.097E+02 | 1.327 | 1.022E-03 | 2.039E+02 |
| 0.166 | 1.018E-03 | 1.012E+04 | 0.961 | 1.028E-02 | 4.733E+02 | 1.336 | 1.273E-02 | 1.348E+03 |
| 0.223 | 9.378E-02 | 1.590E+03 | 0.962 | 1.251E-02 | 2.682E+02 | 1.343 | 4.021E-03 | 1.598E+03 |
| 0.235 | 3.161E-02 | 9.157E+02 | 0.969 | 2.874E-02 | 9.127E-01 | 1.346 | 2.353E-02 | 1.481E+02 |
| 0.245 | 2.179E-02 | 8.402E-01 | 0.972 | 1.309E-05 | 1.216E+02 | 1.347 | 7.485E-04 | 1.438E+03 |
| 0.361 | 4.757E-02 | 3.612E+02 | 0.976 | 2.901E-02 | 1.447E+01 | 1.348 | 1.775E-02 | 7.434E+02 |
| 0.362 | 4.711E-02 | 5.014E+03 | 0.986 | 4.415E-08 | 8.215E+01 | 1.350 | 2.937E-02 | 1.966E+01 |
| 0.369 | 7.819E-02 | 2.929E+00 | 0.988 | 2.824E-02 | 1.349E+02 | 1.361 | 2.456E-02 | 1.368E+03 |
| 0.370 | 7.708E-02 | 3.114E+01 | 0.988 | 1.293E-02 | 1.538E+03 | 1.400 | 6.496E-03 | 5.820E+01 |
| 0.372 | 7.463E-02 | 1.451E+02 | 1.004 | 2.654E-02 | 7.050E+02 | 1.404 | 7.157E-06 | 3.089E+02 |
| 0.373 | 5.287E-02 | 4.708E+02 | 1.021 | 2.546E-02 | 2.288E+03 | 1.407 | 7.592E-03 | 8.560E+01 |
| 0.377 | 6.016E-02 | 5.712E+03 | 1.030 | 1.440E-02 | 2.412E+01 | 1.408 | 2.172E-07 | 1.311E+02 |
| 0.379 | 4.519E-02 | 1.491E+03 | 1.032 | 2.624E-02 | 3.530E+03 | 1.411 | 7.639E-03 | 5.913E+02 |
| 0.379 | 2.047E-02 | 2.573E+02 | 1.042 | 1.618E-02 | 3.722E+02 | 1.486 | 3.344E-02 | 1.402E+03 |
| 0.381 | 7.769E-02 | 2.044E+04 | 1.050 | 1.853E-02 | 2.239E+03 | 1.508 | 8.888E-02 | 9.174E+01 |
| 0.381 | 1.498E-02 | 2.210E+01 | 1.056 | 1.612E-02 | 4.252E+03 | 1.511 | 7.545E-02 | 2.890E+00 |
| 0.386 | 2.297E-02 | 1.539E+03 | 1.065 | 9.647E-02 | 6.558E+02 | 1.512 | 9.941E-02 | 5.651E+02 |
| 0.402 | 4.205E-02 | 4.624E+03 | 1.066 | 9.666E-02 | 2.466E+02 | 1.517 | 1.109E-01 | 1.856E+03 |
| 0.473 | 8.915E-03 | 4.308E+03 | 1.067 | 9.920E-02 | 8.622E+01 | 1.528 | 2.699E-02 | 2.340E+02 |
| 0.499 | 7.879E-03 | 9.899E+02 | 1.070 | 7.817E-02 | 1.697E+03 | 1.574 | 2.684E-02 | 1.240E+02 |

**Supplementary Data for Resonance Strength (continued)**

| Energy (eV) | Width (eV) | Resonance Strength (barn*eV) | Energy (eV) | Width (eV) | Resonance Strength (barn*eV) | Energy (eV) | Width (eV) | Resonance Strength (barn*eV) |
|---|---|---|---|---|---|---|---|---|
| 1.675 | 9.765E-05 | 2.088E+02 | 2.121 | 2.497E-03 | 1.416E+02 | 2.388 | 1.819E-02 | 2.438E+02 |
| 1.684 | 4.326E-03 | 3.704E+01 | 2.129 | 3.223E-04 | 1.808E+02 | 2.394 | 4.911E-04 | 2.949E+02 |
| 1.687 | 1.876E-03 | 5.213E+01 | 2.130 | 9.031E-04 | 5.049E+01 | 2.399 | 1.296E-02 | 5.451E+01 |
| 1.689 | 1.312E-02 | 9.970E+01 | 2.132 | 1.299E-04 | 9.262E+02 | 2.411 | 7.922E-03 | 2.343E+01 |
| 1.691 | 6.569E-03 | 4.824E+01 | 2.133 | 5.370E-05 | 8.358E+02 | 2.413 | 2.898E-02 | 4.600E+00 |
| 1.694 | 2.743E-03 | 4.247E+01 | 2.139 | 3.636E-06 | 1.494E+03 | 2.418 | 1.284E-02 | 1.411E+00 |
| 1.697 | 9.499E-03 | 5.187E+01 | 2.142 | 2.423E-02 | 3.303E+01 | 2.425 | 5.857E-04 | 3.023E+03 |
| 1.709 | 1.711E-04 | 1.194E+03 | 2.144 | 2.163E-02 | 4.648E+00 | 2.430 | 3.531E-02 | 1.484E+03 |
| 1.711 | 7.567E-03 | 2.640E+02 | 2.151 | 2.794E-02 | 1.013E+03 | 2.430 | 6.962E-04 | 1.956E+02 |
| 1.718 | 6.818E-05 | 3.363E+02 | 2.152 | 4.440E-04 | 5.423E+02 | 2.431 | 4.976E-03 | 1.470E+02 |
| 1.723 | 1.766E-04 | 1.163E+03 | 2.152 | 2.295E-02 | 1.590E+02 | 2.431 | 3.122E-02 | 1.001E+02 |
| 1.725 | 5.497E-06 | 8.552E+02 | 2.167 | 1.738E-02 | 3.693E+01 | 2.435 | 2.329E-03 | 1.081E+03 |
| 1.744 | 2.487E-03 | 7.622E+01 | 2.168 | 3.820E-03 | 1.812E+01 | 2.436 | 4.049E-03 | 2.060E+02 |
| 1.753 | 4.236E-04 | 1.093E+02 | 2.170 | 1.172E-02 | 9.131E+02 | 2.441 | 3.470E-03 | 3.918E+02 |
| 1.759 | 4.566E-04 | 1.540E+00 | 2.170 | 4.839E-06 | 1.623E+03 | 2.443 | 3.191E-04 | 7.378E+02 |
| 1.765 | 3.027E-04 | 1.488E+02 | 2.174 | 1.618E-02 | 3.010E+02 | 2.446 | 3.461E-04 | 1.366E+03 |
| 1.806 | 1.327E-03 | 1.363E+01 | 2.176 | 1.137E-06 | 9.593E+02 | 2.452 | 1.903E-03 | 2.394E+02 |
| 1.812 | 1.591E-03 | 3.109E+02 | 2.178 | 1.692E-02 | 3.259E+00 | 2.454 | 1.081E-02 | 7.493E+02 |
| 1.825 | 9.850E-03 | 3.837E+02 | 2.179 | 1.136E-05 | 7.852E+02 | 2.462 | 6.725E-04 | 8.163E+01 |
| 1.839 | 2.625E-04 | 2.148E+00 | 2.184 | 6.325E-07 | 4.042E-13 | 2.472 | 3.086E-03 | 2.781E+02 |
| 1.854 | 2.509E-03 | 1.906E+02 | 2.193 | 6.586E-03 | 1.489E+02 | 2.475 | 4.091E-03 | 1.058E+01 |
| 1.862 | 6.318E-02 | 8.029E+02 | 2.205 | 3.518E-03 | 9.127E+02 | 2.480 | 1.422E-03 | 7.491E+02 |
| 1.873 | 3.254E-02 | 2.578E+02 | 2.209 | 3.877E-03 | 1.231E+03 | 2.482 | 6.874E-03 | 1.268E+01 |
| 1.884 | 5.784E-02 | 6.180E+01 | 2.226 | 7.821E-06 | 9.377E+02 | 2.503 | 9.324E-04 | 6.995E+01 |
| 1.885 | 1.521E-02 | 1.458E+02 | 2.235 | 1.198E-04 | 1.185E+03 | 2.512 | 2.616E-03 | 2.478E+01 |
| 1.909 | 5.091E-02 | 5.738E+02 | 2.238 | 1.115E-06 | 7.989E+02 | 2.515 | 8.582E-04 | 2.569E+02 |
| 1.922 | 8.130E-04 | 1.107E+01 | 2.239 | 3.679E-02 | 6.767E+02 | 2.518 | 8.230E-03 | 5.979E+01 |
| 1.926 | 1.822E-03 | 1.859E+01 | 2.247 | 7.148E-07 | 2.016E+02 | 2.535 | 7.450E-03 | 9.679E+01 |
| 1.928 | 1.172E-06 | 5.433E+01 | 2.249 | 1.544E-05 | 1.047E+03 | 2.544 | 7.088E-03 | 4.959E+02 |
| 1.947 | 1.384E-03 | 1.298E+02 | 2.259 | 1.667E-02 | 6.941E+01 | 2.545 | 4.968E-05 | 4.358E+02 |
| 1.954 | 1.135E-06 | 4.064E+02 | 2.270 | 2.024E-03 | 1.811E+02 | 2.577 | 1.714E-02 | 1.314E+00 |
| 1.970 | 4.235E-03 | 1.214E+02 | 2.271 | 3.484E-02 | 2.307E+01 | 2.579 | 1.398E-02 | 1.168E+01 |
| 1.980 | 9.214E-07 | 1.135E+02 | 2.271 | 3.077E-02 | 1.016E+02 | 2.588 | 7.808E-03 | 1.247E+02 |
| 1.991 | 2.574E-03 | 1.949E+02 | 2.275 | 2.232E-04 | 3.656E+02 | 2.612 | 1.123E-02 | 4.031E+02 |
| 2.005 | 8.805E-07 | 4.119E+00 | 2.280 | 3.051E-02 | 2.677E+01 | 2.622 | 6.934E-03 | 6.901E-01 |
| 2.015 | 2.598E-03 | 5.833E+00 | 2.287 | 3.178E-03 | 1.492E+02 | 2.630 | 5.314E-03 | 5.205E+01 |
| 2.016 | 1.257E-02 | 7.759E+02 | 2.289 | 3.221E-03 | 2.438E-01 | 2.634 | 7.055E-03 | 7.551E+01 |
| 2.021 | 6.440E-02 | 2.650E+02 | 2.304 | 2.496E-03 | 1.724E+02 | 2.634 | 3.434E-03 | 1.701E+02 |
| 2.023 | 6.780E-04 | 1.173E+01 | 2.305 | 2.687E-05 | 1.977E+02 | 2.645 | 7.169E-03 | 1.246E+01 |
| 2.023 | 1.434E-02 | 3.476E+01 | 2.312 | 1.245E-06 | 9.520E+01 | 2.653 | 5.163E-03 | 3.204E+02 |
| 2.044 | 1.568E-03 | 1.940E+02 | 2.314 | 6.160E-04 | 5.937E+02 | 2.654 | 7.677E-04 | 1.668E+01 |
| 2.057 | 6.095E-02 | 5.059E+01 | 2.319 | 7.178E-06 | 2.730E+02 | 2.661 | 7.374E-03 | 3.194E+01 |
| 2.057 | 2.677E-03 | 2.426E+01 | 2.329 | 3.654E-04 | 3.680E+02 | 2.666 | 7.579E-03 | 1.900E+01 |
| 2.077 | 5.712E-04 | 4.410E+02 | 2.350 | 5.001E-03 | 3.374E+01 | 2.667 | 7.229E-03 | 3.429E+01 |
| 2.077 | 3.066E-04 | 3.647E+02 | 2.362 | 2.876E-02 | 5.915E-01 | 2.677 | 2.459E-04 | 1.684E+01 |
| 2.080 | 1.670E-02 | 2.296E+00 | 2.373 | 2.951E-04 | 4.523E+01 | 2.678 | 7.148E-03 | 5.412E-02 |
| 2.089 | 9.905E-02 | 1.334E+03 | 2.380 | 3.994E-04 | 3.178E+02 | 2.682 | 3.124E-03 | 1.273E+01 |
| 2.116 | 6.985E-03 | 6.991E+01 | 2.382 | 5.935E-03 | 9.060E+00 | 2.690 | 6.097E-03 | 2.506E+02 |
| 2.118 | 4.387E-03 | 4.211E+02 | 2.384 | 2.278E-02 | 2.719E+00 | 2.703 | 1.331E-02 | 9.867E-01 |
| 2.121 | 1.062E-03 | 1.308E+02 | 2.387 | 1.667E-02 | 9.895E+02 | 2.705 | 1.452E-02 | 1.325E+02 |

**Supplementary data for the DR cross-section (in barns), with energy given in eV.**

| Energy | Cross section | Energy | Cross section | Energy | Cross section | Energy | Cross section |
|---|---|---|---|---|---|---|---|
| 0.000 | 2.059E+05 | 0.245 | 6.374E+04 | 0.490 | 8.283E+04 | 0.735 | 1.626E+04 |
| 0.005 | 3.152E+05 | 0.250 | 5.977E+04 | 0.495 | 9.217E+04 | 0.740 | 1.490E+04 |
| 0.010 | 5.317E+05 | 0.255 | 5.676E+04 | 0.500 | 9.535E+04 | 0.745 | 1.385E+04 |
| 0.015 | 9.158E+05 | 0.260 | 5.485E+04 | 0.505 | 7.439E+04 | 0.750 | 1.303E+04 |
| 0.020 | 1.31405E6 | 0.265 | 5.385E+04 | 0.510 | 5.541E+04 | 0.755 | 1.237E+04 |
| 0.025 | 1.43289E6 | 0.270 | 5.371E+04 | 0.515 | 4.770E+04 | 0.760 | 1.184E+04 |
| 0.030 | 1.94184E6 | 0.275 | 5.444E+04 | 0.520 | 4.211E+04 | 0.765 | 1.147E+04 |
| 0.035 | 5.30848E6 | 0.280 | 5.596E+04 | 0.525 | 3.608E+04 | 0.770 | 1.126E+04 |
| 0.040 | 1.569E7 | 0.285 | 5.819E+04 | 0.530 | 3.197E+04 | 0.775 | 1.121E+04 |
| 0.045 | 2.74475E7 | 0.290 | 6.116E+04 | 0.535 | 2.948E+04 | 0.780 | 1.139E+04 |
| 0.050 | 2.15974E7 | 0.295 | 6.494E+04 | 0.540 | 2.791E+04 | 0.785 | 1.188E+04 |
| 0.055 | 7.88815E6 | 0.300 | 6.966E+04 | 0.545 | 2.708E+04 | 0.790 | 1.289E+04 |
| 0.060 | 1.83565E6 | 0.305 | 7.546E+04 | 0.550 | 2.686E+04 | 0.795 | 1.461E+04 |
| 0.065 | 6.542E+05 | 0.310 | 8.255E+04 | 0.555 | 2.722E+04 | 0.800 | 1.697E+04 |
| 0.070 | 4.186E+05 | 0.315 | 9.119E+04 | 0.560 | 2.781E+04 | 0.805 | 1.916E+04 |
| 0.075 | 3.324E+05 | 0.320 | 1.017E+05 | 0.565 | 2.853E+04 | 0.810 | 2.050E+04 |
| 0.080 | 2.926E+05 | 0.325 | 1.146E+05 | 0.570 | 3.022E+04 | 0.815 | 2.145E+04 |
| 0.085 | 2.820E+05 | 0.330 | 1.303E+05 | 0.575 | 3.373E+04 | 0.820 | 2.189E+04 |
| 0.090 | 2.940E+05 | 0.335 | 1.495E+05 | 0.580 | 3.990E+04 | 0.825 | 2.035E+04 |
| 0.095 | 3.251E+05 | 0.340 | 1.727E+05 | 0.585 | 4.903E+04 | 0.830 | 1.704E+04 |
| 0.100 | 3.832E+05 | 0.345 | 2.001E+05 | 0.590 | 5.847E+04 | 0.835 | 1.388E+04 |
| 0.105 | 5.234E+05 | 0.350 | 2.312E+05 | 0.595 | 6.217E+04 | 0.840 | 1.177E+04 |
| 0.110 | 1.07108E6 | 0.355 | 2.642E+05 | 0.600 | 5.782E+04 | 0.845 | 1.053E+04 |
| 0.115 | 2.63326E6 | 0.360 | 2.967E+05 | 0.605 | 5.046E+04 | 0.850 | 9.803E+03 |
| 0.120 | 3.87833E6 | 0.365 | 3.258E+05 | 0.610 | 4.548E+04 | 0.855 | 9.379E+03 |
| 0.125 | 3.35777E6 | 0.370 | 3.504E+05 | 0.615 | 4.535E+04 | 0.860 | 9.139E+03 |
| 0.130 | 2.40182E6 | 0.375 | 3.695E+05 | 0.620 | 5.013E+04 | 0.865 | 9.022E+03 |
| 0.135 | 1.586E6 | 0.380 | 3.805E+05 | 0.625 | 5.844E+04 | 0.870 | 8.998E+03 |
| 0.140 | 9.570E+05 | 0.385 | 3.788E+05 | 0.630 | 7.479E+04 | 0.875 | 9.048E+03 |
| 0.145 | 6.141E+05 | 0.390 | 3.623E+05 | 0.635 | 1.163E+05 | 0.880 | 9.166E+03 |
| 0.150 | 5.443E+05 | 0.395 | 3.357E+05 | 0.640 | 2.011E+05 | 0.885 | 9.347E+03 |
| 0.155 | 1.03874E6 | 0.400 | 3.049E+05 | 0.645 | 2.950E+05 | 0.890 | 9.596E+03 |
| 0.160 | 2.49428E6 | 0.405 | 2.722E+05 | 0.650 | 3.457E+05 | 0.895 | 9.924E+03 |
| 0.165 | 2.92999E6 | 0.410 | 2.386E+05 | 0.655 | 3.797E+05 | 0.900 | 1.034E+04 |
| 0.170 | 1.54449E6 | 0.415 | 2.062E+05 | 0.660 | 3.895E+05 | 0.905 | 1.086E+04 |
| 0.175 | 5.499E+05 | 0.420 | 1.772E+05 | 0.665 | 3.558E+05 | 0.910 | 1.155E+04 |
| 0.180 | 2.662E+05 | 0.425 | 1.527E+05 | 0.670 | 3.108E+05 | 0.915 | 1.247E+04 |
| 0.185 | 1.768E+05 | 0.430 | 1.328E+05 | 0.675 | 2.614E+05 | 0.920 | 1.375E+04 |
| 0.190 | 1.323E+05 | 0.435 | 1.169E+05 | 0.680 | 1.998E+05 | 0.925 | 1.568E+04 |
| 0.195 | 1.063E+05 | 0.440 | 1.046E+05 | 0.685 | 1.399E+05 | 0.930 | 1.893E+04 |
| 0.200 | 9.047E+04 | 0.445 | 9.564E+04 | 0.690 | 9.507E+04 | 0.935 | 2.535E+04 |
| 0.205 | 8.080E+04 | 0.450 | 9.052E+04 | 0.695 | 6.655E+04 | 0.940 | 3.858E+04 |
| 0.210 | 7.503E+04 | 0.455 | 9.153E+04 | 0.700 | 4.918E+04 | 0.945 | 5.775E+04 |
| 0.215 | 7.185E+04 | 0.460 | 1.071E+05 | 0.705 | 3.850E+04 | 0.950 | 7.058E+04 |
| 0.220 | 7.062E+04 | 0.465 | 1.583E+05 | 0.710 | 3.172E+04 | 0.955 | 7.254E+04 |
| 0.225 | 7.078E+04 | 0.470 | 2.383E+05 | 0.715 | 2.695E+04 | 0.960 | 7.056E+04 |
| 0.230 | 7.127E+04 | 0.475 | 2.469E+05 | 0.720 | 2.320E+04 | 0.965 | 6.481E+04 |
| 0.235 | 7.057E+04 | 0.480 | 1.653E+05 | 0.725 | 2.023E+04 | 0.970 | 6.296E+04 |
| 0.240 | 6.782E+04 | 0.485 | 1.009E+05 | 0.730 | 1.798E+04 | 0.975 | 6.391E+04 |

**Supplementary data for the DR cross-section (in barns), with energy given in eV (continued).**

| Energy | Cross section | Energy | Cross section | Energy | Cross section | Energy | Cross section |
|---|---|---|---|---|---|---|---|
| 0.980 | 7.597E+04 | 1.225 | 5.140E+04 | 1.470 | 2.713E+04 | 1.715 | 1.040E+05 |
| 0.985 | 1.022E+05 | 1.230 | 3.981E+04 | 1.475 | 3.220E+04 | 1.720 | 1.643E+05 |
| 0.990 | 1.084E+05 | 1.235 | 3.541E+04 | 1.480 | 3.720E+04 | 1.725 | 1.894E+05 |
| 0.995 | 9.520E+04 | 1.240 | 3.188E+04 | 1.485 | 4.030E+04 | 1.730 | 7.298E+04 |
| 1.000 | 8.815E+04 | 1.245 | 2.741E+04 | 1.490 | 4.019E+04 | 1.735 | 1.203E+04 |
| 1.005 | 9.283E+04 | 1.250 | 2.311E+04 | 1.495 | 3.743E+04 | 1.740 | 7.966E+03 |
| 1.010 | 1.063E+05 | 1.255 | 1.986E+04 | 1.500 | 3.383E+04 | 1.745 | 1.090E+04 |
| 1.015 | 1.266E+05 | 1.260 | 1.773E+04 | 1.505 | 3.076E+04 | 1.750 | 1.387E+04 |
| 1.020 | 1.500E+05 | 1.265 | 1.646E+04 | 1.510 | 2.865E+04 | 1.755 | 1.387E+04 |
| 1.025 | 1.705E+05 | 1.270 | 1.582E+04 | 1.515 | 2.743E+04 | 1.760 | 1.334E+04 |
| 1.030 | 1.849E+05 | 1.275 | 1.564E+04 | 1.520 | 2.679E+04 | 1.765 | 1.745E+04 |
| 1.035 | 1.947E+05 | 1.280 | 1.588E+04 | 1.525 | 2.616E+04 | 1.770 | 1.058E+04 |
| 1.040 | 2.088E+05 | 1.285 | 1.659E+04 | 1.530 | 2.488E+04 | 1.775 | 4.700E+03 |
| 1.045 | 2.377E+05 | 1.290 | 1.792E+04 | 1.535 | 2.282E+04 | 1.780 | 3.967E+03 |
| 1.050 | 2.762E+05 | 1.295 | 2.022E+04 | 1.540 | 2.051E+04 | 1.785 | 4.173E+03 |
| 1.055 | 2.939E+05 | 1.300 | 2.424E+04 | 1.545 | 1.843E+04 | 1.790 | 4.534E+03 |
| 1.060 | 2.710E+05 | 1.305 | 3.218E+04 | 1.550 | 1.675E+04 | 1.795 | 5.170E+03 |
| 1.065 | 2.421E+05 | 1.310 | 5.176E+04 | 1.555 | 1.548E+04 | 1.800 | 7.153E+03 |
| 1.070 | 2.455E+05 | 1.315 | 1.067E+05 | 1.560 | 1.458E+04 | 1.805 | 1.551E+04 |
| 1.075 | 2.542E+05 | 1.320 | 2.077E+05 | 1.565 | 1.399E+04 | 1.810 | 3.177E+04 |
| 1.080 | 2.257E+05 | 1.325 | 2.556E+05 | 1.570 | 1.348E+04 | 1.815 | 3.255E+04 |
| 1.085 | 1.764E+05 | 1.330 | 2.004E+05 | 1.575 | 1.272E+04 | 1.820 | 2.504E+04 |
| 1.090 | 1.302E+05 | 1.335 | 1.704E+05 | 1.580 | 1.161E+04 | 1.825 | 2.505E+04 |
| 1.095 | 9.874E+04 | 1.340 | 2.303E+05 | 1.585 | 1.035E+04 | 1.830 | 2.097E+04 |
| 1.100 | 8.652E+04 | 1.345 | 2.989E+05 | 1.590 | 9.216E+03 | 1.835 | 1.541E+04 |
| 1.105 | 8.241E+04 | 1.350 | 2.201E+05 | 1.595 | 8.298E+03 | 1.840 | 1.343E+04 |
| 1.110 | 6.622E+04 | 1.355 | 1.058E+05 | 1.600 | 7.569E+03 | 1.845 | 1.540E+04 |
| 1.115 | 7.511E+04 | 1.360 | 6.846E+04 | 1.605 | 6.979E+03 | 1.850 | 2.346E+04 |
| 1.120 | 1.103E+05 | 1.365 | 5.491E+04 | 1.610 | 6.493E+03 | 1.855 | 2.855E+04 |
| 1.125 | 9.666E+04 | 1.370 | 4.273E+04 | 1.615 | 6.084E+03 | 1.860 | 2.256E+04 |
| 1.130 | 7.415E+04 | 1.375 | 3.260E+04 | 1.620 | 5.735E+03 | 1.865 | 1.872E+04 |
| 1.135 | 1.024E+05 | 1.380 | 2.574E+04 | 1.625 | 5.432E+03 | 1.870 | 1.881E+04 |
| 1.140 | 1.897E+05 | 1.385 | 2.170E+04 | 1.630 | 5.165E+03 | 1.875 | 1.960E+04 |
| 1.145 | 2.325E+05 | 1.390 | 2.023E+04 | 1.635 | 4.933E+03 | 1.880 | 2.036E+04 |
| 1.150 | 1.553E+05 | 1.395 | 2.470E+04 | 1.640 | 4.739E+03 | 1.885 | 2.022E+04 |
| 1.155 | 7.724E+04 | 1.400 | 4.764E+04 | 1.645 | 4.580E+03 | 1.890 | 1.855E+04 |
| 1.160 | 6.167E+04 | 1.405 | 7.569E+04 | 1.650 | 4.461E+03 | 1.895 | 1.649E+04 |
| 1.165 | 1.006E+05 | 1.410 | 6.875E+04 | 1.655 | 4.392E+03 | 1.900 | 1.511E+04 |
| 1.170 | 1.237E+05 | 1.415 | 4.294E+04 | 1.660 | 4.429E+03 | 1.905 | 1.426E+04 |
| 1.175 | 8.721E+04 | 1.420 | 2.438E+04 | 1.665 | 5.736E+03 | 1.910 | 1.350E+04 |
| 1.180 | 7.577E+04 | 1.425 | 1.688E+04 | 1.670 | 1.461E+04 | 1.915 | 1.292E+04 |
| 1.185 | 6.155E+04 | 1.430 | 1.460E+04 | 1.675 | 2.550E+04 | 1.920 | 1.370E+04 |
| 1.190 | 3.347E+04 | 1.435 | 1.404E+04 | 1.680 | 1.967E+04 | 1.925 | 1.631E+04 |
| 1.195 | 3.062E+04 | 1.440 | 1.420E+04 | 1.685 | 1.732E+04 | 1.930 | 1.488E+04 |
| 1.200 | 6.017E+04 | 1.445 | 1.484E+04 | 1.690 | 1.873E+04 | 1.935 | 1.020E+04 |
| 1.205 | 7.880E+04 | 1.450 | 1.593E+04 | 1.695 | 1.682E+04 | 1.940 | 1.107E+04 |
| 1.210 | 7.457E+04 | 1.455 | 1.754E+04 | 1.700 | 2.508E+04 | 1.945 | 2.065E+04 |
| 1.215 | 7.203E+04 | 1.460 | 1.981E+04 | 1.705 | 8.588E+04 | 1.950 | 3.948E+04 |
| 1.220 | 6.461E+04 | 1.465 | 2.295E+04 | 1.710 | 1.318E+05 | 1.955 | 4.577E+04 |

**Supplementary data for the DR cross-section (in barns), with energy given in eV (continued).**

| Energy | Cross section | Energy | Cross section | Energy | Cross section | Energy | Cross section |
|---|---|---|---|---|---|---|---|
| 1.960 | 2.186E+04 | 2.205 | 1.356E+05 | 2.450 | 1.696E+05 | 2.695 | 1.679E+04 |
| 1.965 | 1.247E+04 | 2.210 | 1.305E+05 | 2.455 | 8.152E+04 | 2.700 | 1.443E+04 |
| 1.970 | 1.486E+04 | 2.215 | 6.690E+04 | 2.460 | 4.776E+04 | 2.705 | 1.871E+04 |
| 1.975 | 1.693E+04 | 2.220 | 5.840E+04 | 2.465 | 3.540E+04 | 2.710 | 2.992E+04 |
| 1.980 | 2.024E+04 | 2.225 | 1.101E+05 | 2.470 | 3.994E+04 | 2.715 | 4.022E+04 |
| 1.985 | 1.973E+04 | 2.230 | 1.403E+05 | 2.475 | 6.107E+04 | 2.720 | 3.421E+04 |
| 1.990 | 2.324E+04 | 2.235 | 1.946E+05 | 2.480 | 7.611E+04 | 2.725 | 2.180E+04 |
| 1.995 | 2.018E+04 | 2.240 | 1.540E+05 | 2.485 | 4.226E+04 | 2.730 | 1.650E+04 |
| 2.000 | 1.586E+04 | 2.245 | 1.214E+05 | 2.490 | 1.299E+04 | 2.735 | 1.284E+04 |
| 2.005 | 1.995E+04 | 2.250 | 1.258E+05 | 2.495 | 7.706E+03 | 2.740 | 8.269E+03 |
| 2.010 | 3.019E+04 | 2.255 | 5.315E+04 | 2.500 | 1.037E+04 | 2.745 | 5.632E+03 |
| 2.015 | 3.911E+04 | 2.260 | 1.810E+04 | 2.505 | 1.302E+04 | 2.750 | 4.697E+03 |
| 2.020 | 3.631E+04 | 2.265 | 2.180E+04 | 2.510 | 2.074E+04 | 2.755 | 4.494E+03 |
| 2.025 | 2.597E+04 | 2.270 | 4.147E+04 | 2.515 | 3.071E+04 | 2.760 | 4.670E+03 |
| 2.030 | 1.796E+04 | 2.275 | 5.141E+04 | 2.520 | 1.962E+04 | 2.765 | 5.066E+03 |
| 2.035 | 1.613E+04 | 2.280 | 3.058E+04 | 2.525 | 9.591E+03 | 2.770 | 5.634E+03 |
| 2.040 | 2.271E+04 | 2.285 | 1.917E+04 | 2.530 | 1.070E+04 | 2.775 | 6.412E+03 |
| 2.045 | 2.672E+04 | 2.290 | 1.539E+04 | 2.535 | 1.977E+04 | 2.780 | 7.371E+03 |
| 2.050 | 1.839E+04 | 2.295 | 1.210E+04 | 2.540 | 4.746E+04 | 2.785 | 8.545E+03 |
| 2.055 | 1.386E+04 | 2.300 | 2.458E+04 | 2.545 | 7.057E+04 | 2.790 | 1.022E+04 |
| 2.060 | 1.309E+04 | 2.305 | 4.480E+04 | 2.550 | 3.924E+04 | 2.795 | 1.317E+04 |
| 2.065 | 1.405E+04 | 2.310 | 6.480E+04 | 2.555 | 1.143E+04 | 2.800 | 2.022E+04 |
| 2.070 | 3.202E+04 | 2.315 | 8.130E+04 | 2.560 | 5.164E+03 | 2.805 | 3.619E+04 |
| 2.075 | 7.757E+04 | 2.320 | 5.526E+04 | 2.565 | 3.956E+03 | 2.810 | 4.890E+04 |
| 2.080 | 6.979E+04 | 2.325 | 3.807E+04 | 2.570 | 3.784E+03 | 2.815 | 3.979E+04 |
| 2.085 | 2.655E+04 | 2.330 | 3.795E+04 | 2.575 | 4.346E+03 | 2.820 | 2.828E+04 |
| 2.090 | 1.442E+04 | 2.335 | 1.733E+04 | 2.580 | 6.118E+03 | 2.825 | 2.745E+04 |
| 2.095 | 1.379E+04 | 2.340 | 6.431E+03 | 2.585 | 8.959E+03 | 2.830 | 2.969E+04 |
| 2.100 | 1.443E+04 | 2.345 | 6.359E+03 | 2.590 | 9.689E+03 | 2.835 | 3.775E+04 |
| 2.105 | 1.680E+04 | 2.350 | 7.628E+03 | 2.595 | 8.050E+03 | 2.840 | 5.747E+04 |
| 2.110 | 2.628E+04 | 2.355 | 7.827E+03 | 2.600 | 8.551E+03 | 2.845 | 7.404E+04 |
| 2.115 | 4.991E+04 | 2.360 | 8.435E+03 | 2.605 | 1.312E+04 | 2.850 | 6.545E+04 |
| 2.120 | 6.837E+04 | 2.365 | 1.131E+04 | 2.610 | 1.872E+04 | 2.855 | 4.199E+04 |
| 2.125 | 9.251E+04 | 2.370 | 1.989E+04 | 2.615 | 1.819E+04 | 2.860 | 3.495E+04 |
| 2.130 | 1.978E+05 | 2.375 | 4.059E+04 | 2.620 | 1.325E+04 | 2.865 | 4.350E+04 |
| 2.135 | 2.579E+05 | 2.380 | 6.399E+04 | 2.625 | 1.289E+04 | 2.870 | 4.601E+04 |
| 2.140 | 2.000E+05 | 2.385 | 6.274E+04 | 2.630 | 1.973E+04 | 2.875 | 3.918E+04 |
| 2.145 | 1.005E+05 | 2.390 | 6.448E+04 | 2.635 | 2.208E+04 | 2.880 | 3.759E+04 |
| 2.150 | 8.698E+04 | 2.395 | 6.240E+04 | 2.640 | 1.469E+04 | 2.885 | 3.769E+04 |
| 2.155 | 7.980E+04 | 2.400 | 3.866E+04 | 2.645 | 1.354E+04 | 2.890 | 3.414E+04 |
| 2.160 | 6.444E+04 | 2.405 | 2.613E+04 | 2.650 | 2.226E+04 | 2.895 | 3.535E+04 |
| 2.165 | 1.367E+05 | 2.410 | 2.675E+04 | 2.655 | 2.443E+04 | 2.900 | 5.325E+04 |
| 2.170 | 2.558E+05 | 2.415 | 4.905E+04 | 2.660 | 1.551E+04 | 2.905 | 7.596E+04 |
| 2.175 | 2.629E+05 | 2.420 | 1.749E+05 | 2.665 | 9.876E+03 | 2.910 | 7.165E+04 |
| 2.180 | 1.747E+05 | 2.425 | 3.288E+05 | 2.670 | 7.796E+03 | 2.915 | 5.038E+04 |
| 2.185 | 6.445E+04 | 2.430 | 2.591E+05 | 2.675 | 7.773E+03 | 2.920 | 3.797E+04 |
| 2.190 | 3.089E+04 | 2.435 | 1.977E+05 | 2.680 | 9.717E+03 | 2.925 | 3.896E+04 |
| 2.195 | 3.665E+04 | 2.440 | 2.240E+05 | 2.685 | 1.490E+04 | 2.930 | 3.418E+04 |
| 2.200 | 7.376E+04 | 2.445 | 2.584E+05 | 2.690 | 1.965E+04 | 2.935 | 2.156E+04 |

**Supplementary data for the DR cross-section (in barns), with energy given in eV (continued).**

| Energy | Cross section | Energy | Cross section | Energy | Cross section | Energy | Cross section |
|---|---|---|---|---|---|---|---|
| 2.940 | 1.277E+04 | 3.185 | 4.297E+03 | 3.430 | 2.413E+03 | 3.675 | 4.742E+03 |
| 2.945 | 9.171E+03 | 3.190 | 4.665E+03 | 3.435 | 2.498E+03 | 3.680 | 4.668E+03 |
| 2.950 | 8.080E+03 | 3.195 | 5.208E+03 | 3.440 | 2.607E+03 | 3.685 | 4.610E+03 |
| 2.955 | 8.027E+03 | 3.200 | 5.868E+03 | 3.445 | 2.747E+03 | 3.690 | 4.567E+03 |
| 2.960 | 8.272E+03 | 3.205 | 6.784E+03 | 3.450 | 2.930E+03 | 3.695 | 4.544E+03 |
| 2.965 | 8.764E+03 | 3.210 | 8.259E+03 | 3.455 | 3.172E+03 | 3.700 | 4.548E+03 |
| 2.970 | 9.297E+03 | 3.215 | 9.083E+03 | 3.460 | 3.486E+03 | 3.705 | 4.588E+03 |
| 2.975 | 9.668E+03 | 3.220 | 7.749E+03 | 3.465 | 3.852E+03 | 3.710 | 4.667E+03 |
| 2.980 | 1.046E+04 | 3.225 | 5.892E+03 | 3.470 | 4.203E+03 | 3.715 | 4.784E+03 |
| 2.985 | 1.236E+04 | 3.230 | 4.946E+03 | 3.475 | 4.476E+03 | 3.720 | 4.945E+03 |
| 2.990 | 1.725E+04 | 3.235 | 4.687E+03 | 3.480 | 4.651E+03 | 3.725 | 5.166E+03 |
| 2.995 | 2.061E+04 | 3.240 | 4.759E+03 | 3.485 | 4.722E+03 | 3.730 | 5.436E+03 |
| 3.000 | 2.158E+04 | 3.245 | 4.988E+03 | 3.490 | 4.713E+03 | 3.735 | 5.620E+03 |
| 3.005 | 2.572E+04 | 3.250 | 5.224E+03 | 3.495 | 4.690E+03 | 3.740 | 5.572E+03 |
| 3.010 | 3.130E+04 | 3.255 | 5.220E+03 | 3.500 | 4.733E+03 | 3.745 | 5.383E+03 |
| 3.015 | 4.112E+04 | 3.260 | 5.200E+03 | 3.505 | 4.855E+03 | 3.750 | 5.237E+03 |
| 3.020 | 5.397E+04 | 3.265 | 5.564E+03 | 3.510 | 4.961E+03 | 3.755 | 5.192E+03 |
| 3.025 | 6.689E+04 | 3.270 | 5.940E+03 | 3.515 | 4.935E+03 | 3.760 | 5.228E+03 |
| 3.030 | 7.832E+04 | 3.275 | 5.617E+03 | 3.520 | 4.753E+03 | 3.765 | 5.326E+03 |
| 3.035 | 8.162E+04 | 3.280 | 4.742E+03 | 3.525 | 4.545E+03 | 3.770 | 5.476E+03 |
| 3.040 | 7.392E+04 | 3.285 | 4.010E+03 | 3.530 | 4.431E+03 | 3.775 | 5.680E+03 |
| 3.045 | 6.072E+04 | 3.290 | 3.657E+03 | 3.535 | 4.425E+03 | 3.780 | 5.949E+03 |
| 3.050 | 5.210E+04 | 3.295 | 3.625E+03 | 3.540 | 4.498E+03 | 3.785 | 6.296E+03 |
| 3.055 | 5.093E+04 | 3.300 | 4.103E+03 | 3.545 | 4.611E+03 | 3.790 | 6.660E+03 |
| 3.060 | 4.865E+04 | 3.305 | 5.456E+03 | 3.550 | 4.723E+03 | 3.795 | 6.858E+03 |
| 3.065 | 3.965E+04 | 3.310 | 6.759E+03 | 3.555 | 4.812E+03 | 3.800 | 6.836E+03 |
| 3.070 | 3.222E+04 | 3.315 | 6.137E+03 | 3.560 | 4.884E+03 | 3.805 | 6.801E+03 |
| 3.075 | 3.231E+04 | 3.320 | 4.614E+03 | 3.565 | 4.963E+03 | 3.810 | 6.927E+03 |
| 3.080 | 3.424E+04 | 3.325 | 3.935E+03 | 3.570 | 5.052E+03 | 3.815 | 7.188E+03 |
| 3.085 | 2.925E+04 | 3.330 | 4.213E+03 | 3.575 | 5.137E+03 | 3.820 | 7.354E+03 |
| 3.090 | 2.023E+04 | 3.335 | 5.475E+03 | 3.580 | 5.218E+03 | 3.825 | 7.315E+03 |
| 3.095 | 1.396E+04 | 3.340 | 8.029E+03 | 3.585 | 5.325E+03 | 3.830 | 7.278E+03 |
| 3.100 | 1.117E+04 | 3.345 | 1.090E+04 | 3.590 | 5.517E+03 | 3.835 | 7.379E+03 |
| 3.105 | 1.037E+04 | 3.350 | 1.110E+04 | 3.595 | 5.886E+03 | 3.840 | 7.618E+03 |
| 3.110 | 1.040E+04 | 3.355 | 8.338E+03 | 3.600 | 6.420E+03 | 3.845 | 8.028E+03 |
| 3.115 | 1.030E+04 | 3.360 | 5.619E+03 | 3.605 | 6.788E+03 | 3.850 | 8.788E+03 |
| 3.120 | 9.943E+03 | 3.365 | 4.132E+03 | 3.610 | 6.668E+03 | 3.855 | 1.004E+04 |
| 3.125 | 9.832E+03 | 3.370 | 3.365E+03 | 3.615 | 6.277E+03 | 3.860 | 1.102E+04 |
| 3.130 | 9.482E+03 | 3.375 | 2.910E+03 | 3.620 | 5.976E+03 | 3.865 | 1.090E+04 |
| 3.135 | 8.157E+03 | 3.380 | 2.648E+03 | 3.625 | 5.831E+03 | 3.870 | 1.055E+04 |
| 3.140 | 6.653E+03 | 3.385 | 2.516E+03 | 3.630 | 5.755E+03 | 3.875 | 1.022E+04 |
| 3.145 | 5.668E+03 | 3.390 | 2.430E+03 | 3.635 | 5.685E+03 | 3.880 | 9.385E+03 |
| 3.150 | 5.107E+03 | 3.395 | 2.346E+03 | 3.640 | 5.597E+03 | 3.885 | 8.214E+03 |
| 3.155 | 4.737E+03 | 3.400 | 2.281E+03 | 3.645 | 5.484E+03 | 3.890 | 7.162E+03 |
| 3.160 | 4.451E+03 | 3.405 | 2.250E+03 | 3.650 | 5.353E+03 | 3.895 | 6.464E+03 |
| 3.165 | 4.232E+03 | 3.410 | 2.247E+03 | 3.655 | 5.213E+03 | 3.900 | 6.127E+03 |
| 3.170 | 4.090E+03 | 3.415 | 2.263E+03 | 3.660 | 5.074E+03 | 3.905 | 6.076E+03 |
| 3.175 | 4.040E+03 | 3.420 | 2.296E+03 | 3.665 | 4.945E+03 | 3.910 | 6.243E+03 |
| 3.180 | 4.101E+03 | 3.425 | 2.346E+03 | 3.670 | 4.834E+03 | 3.915 | 6.580E+03 |

**Supplementary data for the DR cross-section (in barns), with energy given in eV (continued).**

| Energy | Cross section | Energy | Cross section | Energy | Cross section | Energy | Cross section |
|---|---|---|---|---|---|---|---|
| 3.920 | 7.049E+03 | 4.165 | 3.361E+03 | 4.410 | 4.185E+03 | 4.655 | 3.113E+03 |
| 3.925 | 7.634E+03 | 4.170 | 3.315E+03 | 4.415 | 4.165E+03 | 4.660 | 3.161E+03 |
| 3.930 | 8.303E+03 | 4.175 | 3.279E+03 | 4.420 | 4.158E+03 | 4.665 | 3.217E+03 |
| 3.935 | 8.929E+03 | 4.180 | 3.250E+03 | 4.425 | 4.160E+03 | 4.670 | 3.281E+03 |
| 3.940 | 9.422E+03 | 4.185 | 3.227E+03 | 4.430 | 4.168E+03 | 4.675 | 3.353E+03 |
| 3.945 | 9.912E+03 | 4.190 | 3.209E+03 | 4.435 | 4.178E+03 | 4.680 | 3.433E+03 |
| 3.950 | 1.053E+04 | 4.195 | 3.196E+03 | 4.440 | 4.189E+03 | 4.685 | 3.521E+03 |
| 3.955 | 1.121E+04 | 4.200 | 3.187E+03 | 4.445 | 4.197E+03 | 4.690 | 3.617E+03 |
| 3.960 | 1.173E+04 | 4.205 | 3.182E+03 | 4.450 | 4.200E+03 | 4.695 | 3.722E+03 |
| 3.965 | 1.190E+04 | 4.210 | 3.182E+03 | 4.455 | 4.197E+03 | 4.700 | 3.836E+03 |
| 3.970 | 1.163E+04 | 4.215 | 3.185E+03 | 4.460 | 4.185E+03 | 4.705 | 3.961E+03 |
| 3.975 | 1.099E+04 | 4.220 | 3.192E+03 | 4.465 | 4.163E+03 | 4.710 | 4.097E+03 |
| 3.980 | 1.015E+04 | 4.225 | 3.201E+03 | 4.470 | 4.132E+03 | 4.715 | 4.247E+03 |
| 3.985 | 9.296E+03 | 4.230 | 3.212E+03 | 4.475 | 4.091E+03 | 4.720 | 4.410E+03 |
| 3.990 | 8.547E+03 | 4.235 | 3.225E+03 | 4.480 | 4.042E+03 | 4.725 | 4.590E+03 |
| 3.995 | 7.966E+03 | 4.240 | 3.238E+03 | 4.485 | 3.988E+03 | 4.730 | 4.786E+03 |
| 4.000 | 7.563E+03 | 4.245 | 3.252E+03 | 4.490 | 3.930E+03 | 4.735 | 5.001E+03 |
| 4.005 | 7.331E+03 | 4.250 | 3.266E+03 | 4.495 | 3.871E+03 | 4.740 | 5.235E+03 |
| 4.010 | 7.253E+03 | 4.255 | 3.279E+03 | 4.500 | 3.814E+03 | 4.745 | 5.488E+03 |
| 4.015 | 7.319E+03 | 4.260 | 3.293E+03 | 4.505 | 3.763E+03 | 4.750 | 5.759E+03 |
| 4.020 | 7.727E+03 | 4.265 | 3.306E+03 | 4.510 | 3.720E+03 | 4.755 | 6.047E+03 |
| 4.025 | 8.718E+03 | 4.270 | 3.319E+03 | 4.515 | 3.691E+03 | 4.760 | 6.349E+03 |
| 4.030 | 9.642E+03 | 4.275 | 3.333E+03 | 4.520 | 3.679E+03 | 4.765 | 6.659E+03 |
| 4.035 | 9.175E+03 | 4.280 | 3.347E+03 | 4.525 | 3.687E+03 | 4.770 | 6.971E+03 |
| 4.040 | 7.488E+03 | 4.285 | 3.362E+03 | 4.530 | 3.711E+03 | 4.775 | 7.277E+03 |
| 4.045 | 5.900E+03 | 4.290 | 3.379E+03 | 4.535 | 3.741E+03 | 4.780 | 7.565E+03 |
| 4.050 | 4.914E+03 | 4.295 | 3.399E+03 | 4.540 | 3.775E+03 | 4.785 | 7.825E+03 |
| 4.055 | 4.356E+03 | 4.300 | 3.424E+03 | 4.545 | 3.806E+03 | 4.790 | 8.050E+03 |
| 4.060 | 4.028E+03 | 4.305 | 3.454E+03 | 4.550 | 3.811E+03 | 4.795 | 8.237E+03 |
| 4.065 | 3.825E+03 | 4.310 | 3.490E+03 | 4.555 | 3.802E+03 | 4.800 | 8.391E+03 |
| 4.070 | 3.698E+03 | 4.315 | 3.535E+03 | 4.560 | 3.791E+03 | 4.805 | 8.512E+03 |
| 4.075 | 3.621E+03 | 4.320 | 3.589E+03 | 4.565 | 3.762E+03 | 4.810 | 8.608E+03 |
| 4.080 | 3.581E+03 | 4.325 | 3.655E+03 | 4.570 | 3.708E+03 | 4.815 | 8.694E+03 |
| 4.085 | 3.567E+03 | 4.330 | 3.734E+03 | 4.575 | 3.638E+03 | 4.820 | 8.786E+03 |
| 4.090 | 3.576E+03 | 4.335 | 3.831E+03 | 4.580 | 3.569E+03 | 4.825 | 8.887E+03 |
| 4.095 | 3.608E+03 | 4.340 | 3.944E+03 | 4.585 | 3.505E+03 | 4.830 | 8.993E+03 |
| 4.100 | 3.679E+03 | 4.345 | 4.069E+03 | 4.590 | 3.442E+03 | 4.835 | 9.099E+03 |
| 4.105 | 3.819E+03 | 4.350 | 4.189E+03 | 4.595 | 3.368E+03 | 4.840 | 9.197E+03 |
| 4.110 | 3.957E+03 | 4.355 | 4.277E+03 | 4.600 | 3.282E+03 | 4.845 | 9.282E+03 |
| 4.115 | 3.944E+03 | 4.360 | 4.325E+03 | 4.605 | 3.193E+03 | 4.850 | 9.349E+03 |
| 4.120 | 3.862E+03 | 4.365 | 4.355E+03 | 4.610 | 3.116E+03 | 4.855 | 9.396E+03 |
| 4.125 | 3.845E+03 | 4.370 | 4.402E+03 | 4.615 | 3.059E+03 | 4.860 | 9.422E+03 |
| 4.130 | 3.912E+03 | 4.375 | 4.506E+03 | 4.620 | 3.022E+03 | 4.865 | 9.430E+03 |
| 4.135 | 4.064E+03 | 4.380 | 4.678E+03 | 4.625 | 3.002E+03 | 4.870 | 9.427E+03 |
| 4.140 | 4.135E+03 | 4.385 | 4.800E+03 | 4.630 | 2.996E+03 | 4.875 | 9.418E+03 |
| 4.145 | 3.936E+03 | 4.390 | 4.707E+03 | 4.635 | 3.001E+03 | 4.880 | 9.412E+03 |
| 4.150 | 3.673E+03 | 4.395 | 4.488E+03 | 4.640 | 3.016E+03 | 4.885 | 9.414E+03 |
| 4.155 | 3.513E+03 | 4.400 | 4.320E+03 | 4.645 | 3.040E+03 | 4.890 | 9.428E+03 |
| 4.160 | 3.422E+03 | 4.405 | 4.229E+03 | 4.650 | 3.072E+03 | 4.895 | 9.454E+03 |

**Supplementary data for the DR cross-section (in barns), with energy given in eV (continued).**

| Energy | Cross section |
|---|---|
| 4.900 | 9.483E+03 |
| 4.905 | 9.498E+03 |
| 4.910 | 9.480E+03 |
| 4.915 | 9.412E+03 |
| 4.920 | 9.281E+03 |
| 4.925 | 9.087E+03 |
| 4.930 | 8.835E+03 |
| 4.935 | 8.532E+03 |
| 4.940 | 8.193E+03 |
| 4.945 | 7.835E+03 |
| 4.950 | 7.476E+03 |
| 4.955 | 7.129E+03 |
| 4.960 | 6.801E+03 |
| 4.965 | 6.497E+03 |
| 4.970 | 6.218E+03 |
| 4.975 | 5.961E+03 |
| 4.980 | 5.725E+03 |
| 4.985 | 5.506E+03 |
| 4.990 | 5.300E+03 |
| 4.995 | 5.106E+03 |
| 5.000 | 4.920E+03 |

**Supplementary Data for DR Rate Coefficients**

| Temperature (K) | Rate coefficient (cm$^3$/s) | Temperature (K) | Rate coefficient (cm$^3$/s) |
|---|---|---|---|
| 2 | 7.49E-64 | 600000 | 5.95E-14 |
| 3 | 1.23E-45 | 700000 | 4.75E-14 |
| 4 | 1.39E-36 | 800000 | 3.91E-14 |
| 5 | 3.47E-31 | 900000 | 3.28E-14 |
| 6 | 1.31E-27 | 1000000 | 2.81E-14 |
| 7 | 4.54E-25 | 2E6 | 1.01E-14 |
| 8 | 3.54E-23 | 3E6 | 5.5E-15 |
| 9 | 1.03E-21 | 4E6 | 3.58E-15 |
| 10 | 1.5E-20 | 5E6 | 2.57E-15 |
| 20 | 1.86E-15 | 6E6 | 1.95E-15 |
| 30 | 7.16E-14 | 7E6 | 1.55E-15 |
| 40 | 4.04E-13 | 8E6 | 1.27E-15 |
| 50 | 1.13E-12 | 9E6 | 1.06E-15 |
| 60 | 2.34E-12 | 1E7 | 9.09E-16 |
| 70 | 4.1E-12 | 2E7 | 3.22E-16 |
| 80 | 6.45E-12 | 3E7 | 1.75E-16 |
| 90 | 9.34E-12 | 4E7 | 1.14E-16 |
| 100 | 1.27E-11 | 5E7 | 8.15E-17 |
| 200 | 4.59E-11 | 6E7 | 6.2E-17 |
| 300 | 5.92E-11 | 7E7 | 4.92E-17 |
| 400 | 6.13E-11 | 8E7 | 4.03E-17 |
| 500 | 5.94E-11 | 9E7 | 3.38E-17 |
| 600 | 5.61E-11 | 1E8 | 2.88E-17 |
| 700 | 5.25E-11 | 2E8 | 1.02E-17 |
| 800 | 4.91E-11 | 3E8 | 5.55E-18 |
| 900 | 4.58E-11 | 4E8 | 3.6E-18 |
| 1000 | 4.28E-11 | 5E8 | 2.58E-18 |
| 2000 | 2.51E-11 | 6E8 | 1.96E-18 |
| 3000 | 1.77E-11 | 7E8 | 1.56E-18 |
| 4000 | 1.38E-11 | 8E8 | 1.27E-18 |
| 5000 | 1.15E-11 | 9E8 | 1.07E-18 |
| 6000 | 9.92E-12 | 1E9 | 9.12E-19 |
| 7000 | 8.82E-12 | 2E9 | 3.22E-19 |
| 8000 | 7.99E-12 | 3E9 | 1.75E-19 |
| 9000 | 7.33E-12 | 4E9 | 1.14E-19 |
| 10000 | 6.8E-12 | 5E9 | 8.15E-20 |
| 20000 | 4.04E-12 | 6E9 | 6.2E-20 |
| 30000 | 2.82E-12 | 7E9 | 4.92E-20 |
| 40000 | 2.11E-12 | 8E9 | 4.03E-20 |
| 50000 | 1.66E-12 | 9E9 | 3.38E-20 |
| 60000 | 1.35E-12 | 1E10 | 2.88E-20 |
| 70000 | 1.12E-12 | 2E10 | 1.02E-20 |
| 80000 | 9.55E-13 | 3E10 | 5.55E-21 |
| 90000 | 8.25E-13 | 4E10 | 3.6E-21 |
| 100000 | 7.21E-13 | 5E10 | 2.58E-21 |
| 200000 | 2.86E-13 | 6E10 | 1.96E-21 |
| 300000 | 1.62E-13 | 7E10 | 1.56E-21 |
| 400000 | 1.07E-13 | 8E10 | 1.27E-21 |
| 500000 | 7.76E-14 | 9E10 | 1.07E-21 |
| | | 1E11 | 9.12E-22 |
